# Supplementary material for: Multimodal Motion Conditioned Diffusion Model for Skeleton-based Video Anomaly Detection
Source: arXiv:2307.07205 source file (2023-08-28)
Supplement: Supplementary file 1 [file 8_visualization_appendix.tex]

\begin{figure*}[ht]
    \centering
    \begin{subfigure}[b]{0.48\linewidth}
    \centering
    \includegraphics[width=\linewidth]{iccv2023AuthorKit/Images/attempts/normal_sample_barplot.pdf}
    \caption{}
    \label{subfig:normal_barplot}
    \end{subfigure}
    \begin{subfigure}[b]{0.48\linewidth}
    \centering
    \includegraphics[width=\linewidth]{iccv2023AuthorKit/Images/attempts/anomalous_sample_barplot.pdf}
    \caption{}
    \label{subfig:anomalous_barplot}
    \end{subfigure}
    \caption{Visualization of the displacement error values when generating 50 times for each sample of the UBnormal test set. Colored bars show the distribution for a randomly chosen realization, sampled from the normal and abnormal classes (\ref{subfig:normal_barplot} and \ref{subfig:anomalous_barplot}, respectively). The gray bars refer to the average distribution of the displacement error values. The generations are sorted from the best to the worst. The $i$-th number on the x-axis refers to the index of the $i$-th generation. The error values are reported in the log scale}
    \label{fig:normal_anomalous_barplots}
\end{figure*}

\begin{figure*}[ht]
    \centering
    \begin{subfigure}[b]{0.48\linewidth}
    \centering
    \includegraphics[width=\linewidth]{iccv2023AuthorKit/Images/attempts/normal_sample.pdf}
    \caption{}
    \label{subfig:normal_sample_discarded}
    \end{subfigure}
    \begin{subfigure}[b]{0.48\linewidth}
    \centering
    \includegraphics[width=\linewidth]{iccv2023AuthorKit/Images/attempts/anomalous_sample.pdf}
    \caption{}
    \label{subfig:anomalous_sample_discarded}
    \end{subfigure}
    \caption{Visualization of the displacement\FG{"reconstruction"?} \AF{concordo. displacement error si riferisce alla loss usata solo a train} error's \textit{probability density function} (PDF) when generating 50 times for each sample of the UBnormal test set. Colored bars refer to the PDF for a randomly chosen realization, sampled from the normal and abnormal classes (\ref{subfig:normal_sample_discarded} and \ref{subfig:anomalous_sample_discarded}, respectively). In both plots, the dashed line highlights their $0.1$ quantile. The gray bars depict the displacement error's PDF across all the samples in the set, whereas the gray line is its \textit{kernel density estimate} (KDE). Note that the error values are reported in the log scale.
    \FG{For discussion: (1) if we trust the distribution, then a single random sample should have its shape, or we're cheating. Sorry maybe I gave the wrong suggestion yesterday.. let me try to improve it; (2) what about trying a tSNE or anyhow dimensionality reduction to 2 dimensions? One may depict GT in the middle and (maybe) the multiple modes of the generated samples (a dot for each sample); (3) the very last plot in the discord thread "visualizzazione delle distribuzioni", the one superposing pink/light blue for normal vs anomalous seems best, also for explaining, as it shows that the anomalous distribution is much more spread (need to emphasize it in the description); (4) why log scale? it makes the anomalous look much closer to a 0 error. Without log scale one would see the negative drop earlier, incapable of reaching the actual GT even after lots of sampling.}
    }
    \label{fig:normal_anomalous_distros_discarded}
\end{figure*}

\newpage

\begin{figure*}[!ht]
    \begin{center}
\includegraphics[width=0.9\linewidth]{Images/Pictorial_w_t.pdf}
    \caption{\TD{choice}}
    \label{fig:architecture2}
    \end{center}
\end{figure*}

\begin{figure*}[!ht]
    \begin{center}
\includegraphics[width=0.9\linewidth]{Images/Pictorial_w_latents.pdf}
    \caption{\TD{choice.}\AF{ I like this one more with latent vectors, but it'd be better if the yellow one doesn't touch the inject line (latent format da soli 4 quadrati invece di 6?). Maybe the blue latent vector is not needed. \_rec and \_disp are difficult to read }}
    \label{fig:architecture3}
    \end{center}
\end{figure*}
