# Supplementary material for: Multimodal Motion Conditioned Diffusion Model for Skeleton-based Video Anomaly Detection
Source: arXiv:2307.07205 source file (2023-08-28)
Supplement: Supplementary file 2 [file metrics.tex]

\begin{figure*}[ht]
    \centering
    \begin{subfigure}[b]{0.48\linewidth}
    \centering
    \includegraphics[width=\linewidth]{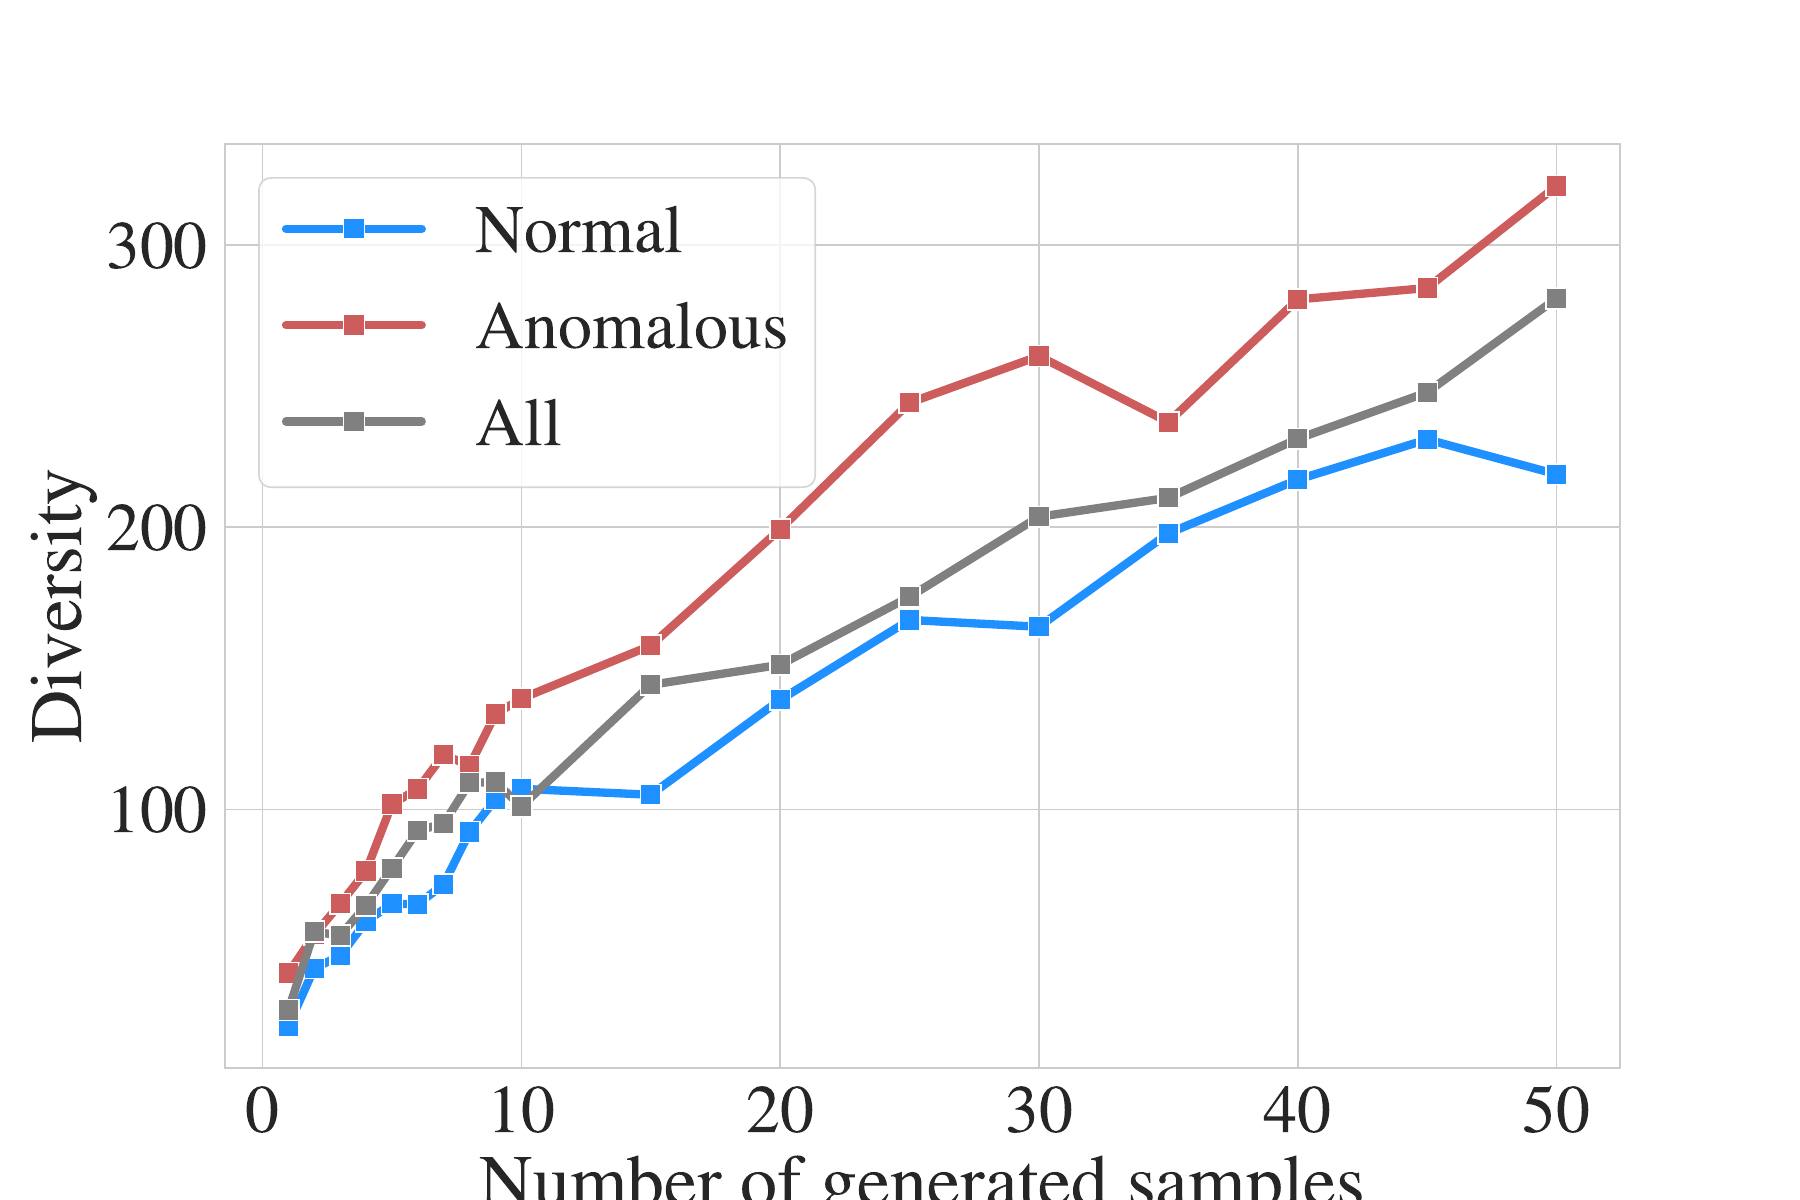}
    % \caption{}
    % \label{subfig:average_normal_anomalous_distro}
    \end{subfigure}
    \begin{subfigure}[b]{0.48\linewidth}
    \centering
    \includegraphics[width=\linewidth]{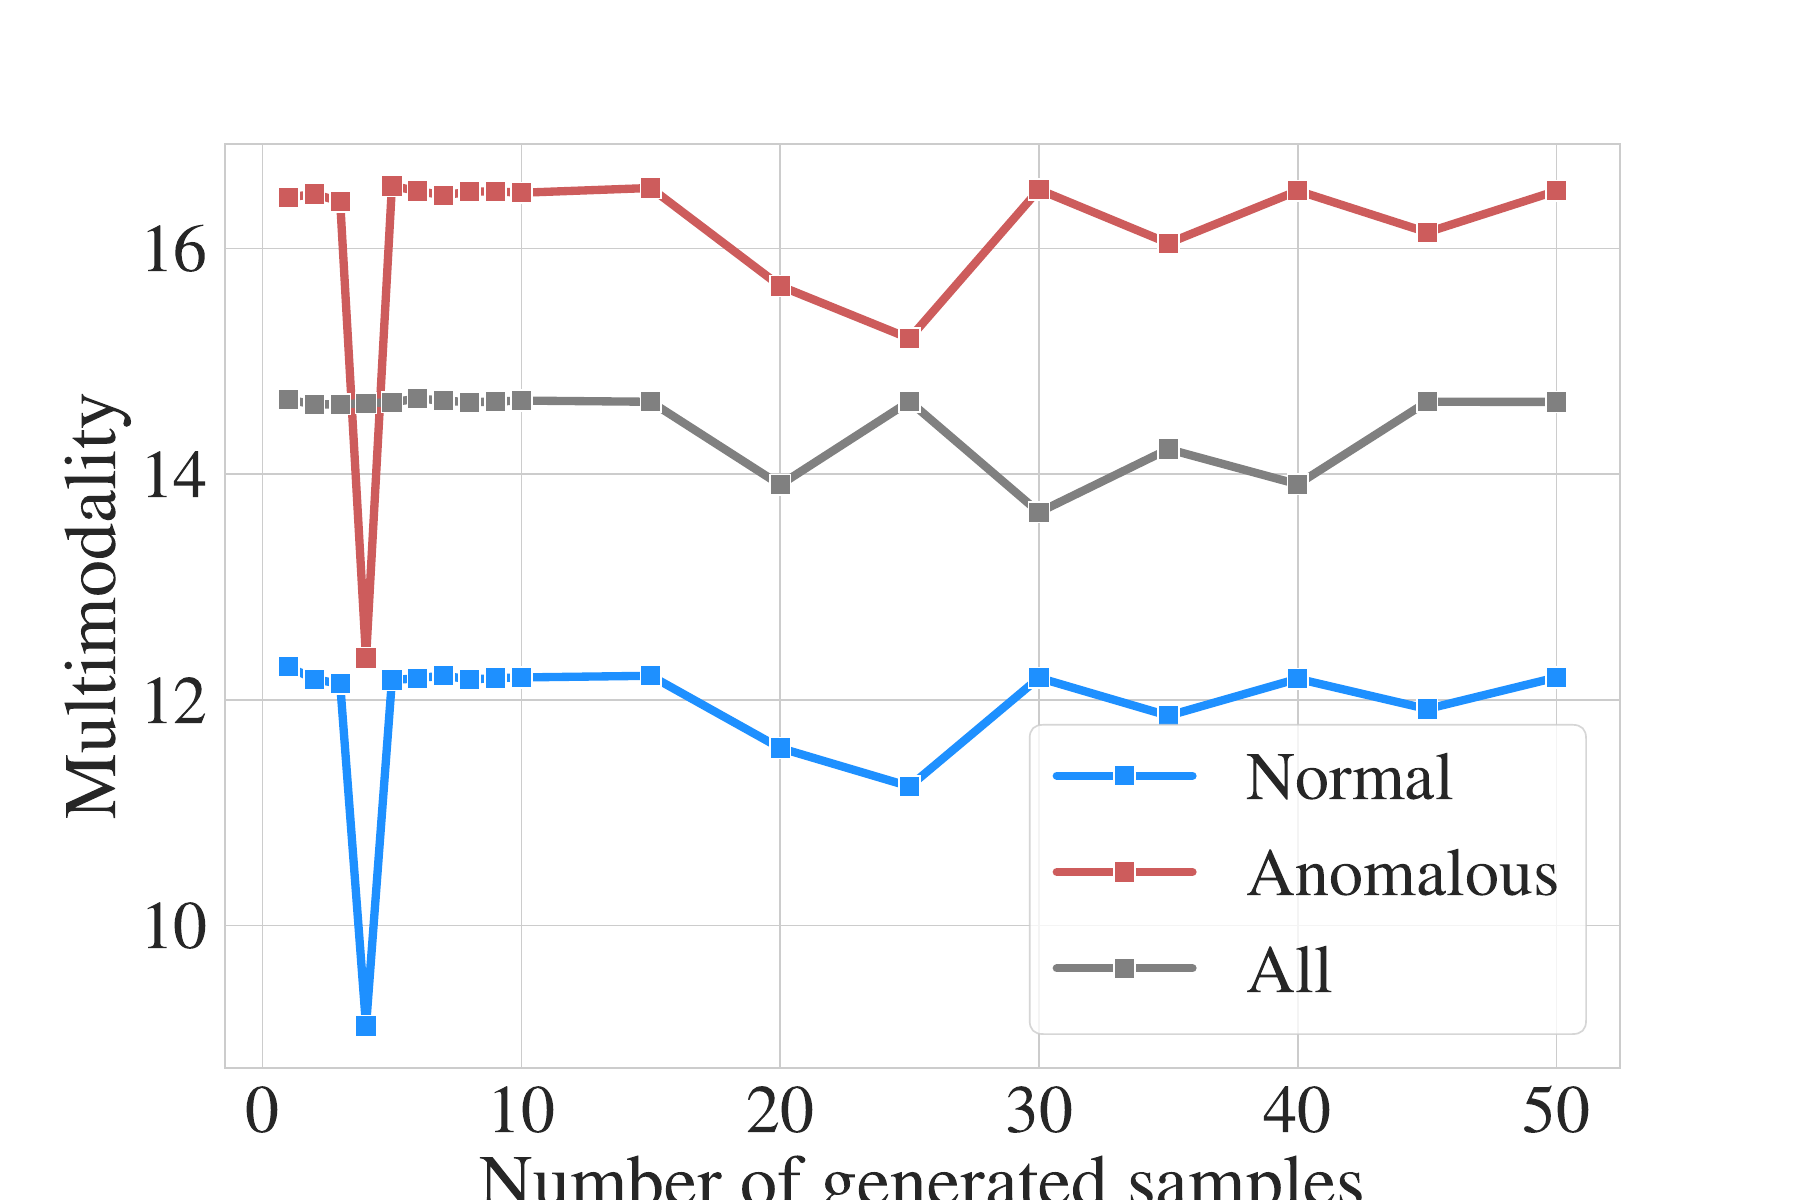}
    % \caption{}
    % \label{subfig:auc_trend}
    \end{subfigure}
    \caption{
    (\textit{left}) Diversity.
    (\textit{right}) Multimodality.
    % \ref{subfig:average_normal_anomalous_distro} Visualization of the average reconstruction error's \textit{probability density function} (PDF) when generating 50 times for each sample of the UBnormal test set. For each sample, the 50 generations have been sorted from the best to the worst in terms of error and averaged across the samples. The solid lines represent their \textit{kernel density estimate} (KDE).
    % \ref{subfig:auc_trend} Correlation between the AUC scores and the number of generations, with each curve corresponding to a different function used to aggregate multiple generations.
    }
    \label{fig:metrics}

\end{figure*}
