# Supplementary material for: Multimodal Motion Conditioned Diffusion Model for Skeleton-based Video Anomaly Detection
Source: arXiv:2307.07205 source file (2023-08-28)
Supplement: Supplementary file 3 [file viz_ale.tex]

\begin{figure}[t]
\vspace*{-2mm}
\begin{center}
	\includegraphics[width=\linewidth]{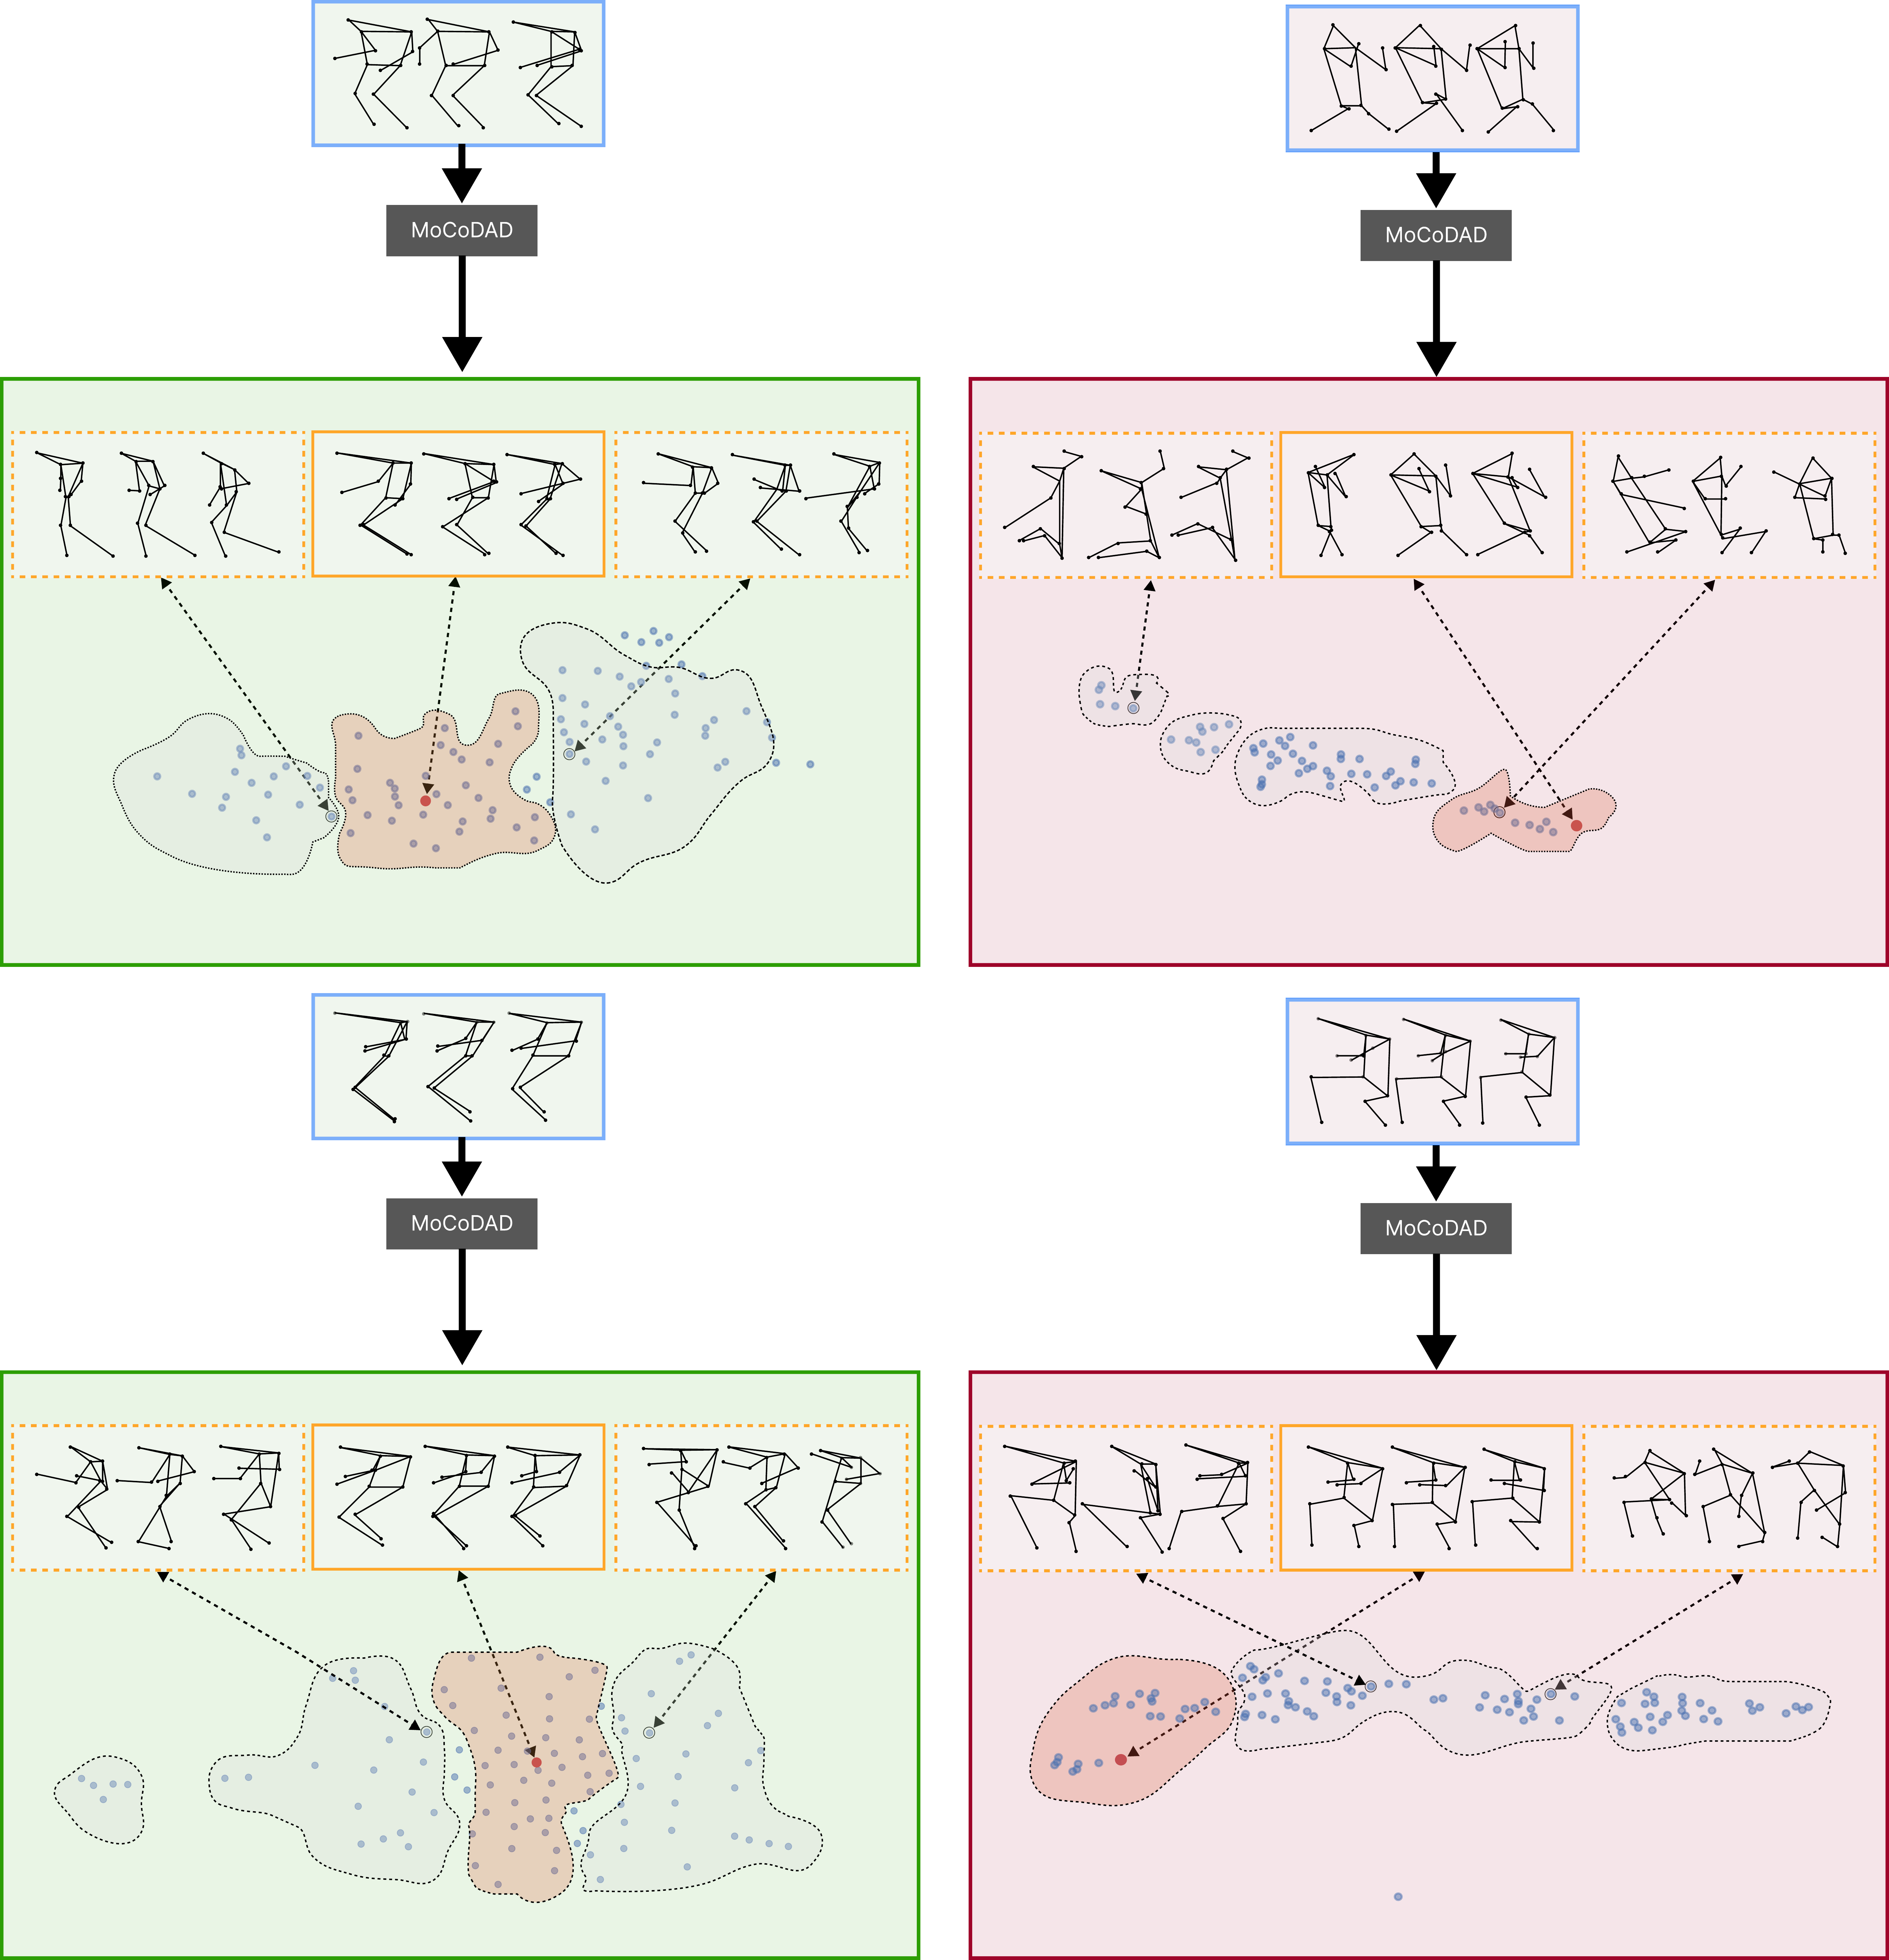}
\end{center}
\vspace*{-5mm}
\caption{Comparison of Gaussian vs Simplex Noise}
\vspace*{-4mm}

\label{fig:simplexvsgaus}
\end{figure}
