# Supplementary material for: Multimodal Motion Conditioned Diffusion Model for Skeleton-based Video Anomaly Detection
Source: arXiv:2307.07205 source file (2023-08-28)
Supplement: Supplementary file 4 [file chance_level.tex]

\begin{table}[h]
\centering{%
\caption{chance level}
\label{tab:chance}

\begin{tabular}{lcc}
\toprule

  & \textbf{UBnormal} & \textbf{HR-UBnormal}\\ 
\midrule
\midrule
 % \hline
 Constant & 49.50 &   \\
 Random Loss & 49.60 & \\
w/o Motion Condition    &  54.11 &   54.98    \\
 MoCoDAD  & \textbf{\ubnres} &  \textbf{\hrubnres}      \\

\bottomrule
\end{tabular}}

\end{table}
