# Supplementary material for: Multimodal Motion Conditioned Diffusion Model for Skeleton-based Video Anomaly Detection
Source: arXiv:2307.07205 source file (2023-08-28)
Supplement: Supplementary file 5 [file metrics.tex]

\begin{table*}[h]
\centering{%
\caption{Diversity metrics for 50 generations.}
\label{tab:metrics}

\begin{tabular}{l|ccc|ccc|ccc}
\toprule
& \multicolumn{3}{c|}{\textbf{Diversity} $\rightarrow$} & \multicolumn{3}{c|}{\textbf{Multimodality} $\uparrow$} & \multicolumn{3}{c}{\textbf{rF} $\uparrow$}\\
& Normal & Abnormal & All & Normal & Abnormal & All & Normal & Abnormal & All\\ 
\midrule
\textbf{Real motions} & 8.07 & 9.90 & 9.16 & - & - & - & - & - & -\\
\midrule
 \OUR+MLD  & 143.66 & 144.68 & 144.78 & 15.48 & 15.56 & 15.52 & 10.02 & 8.82 & 9.33 \\
 Latent-\OUR & 56.27 & 71.35 & 61.32 & - & - & - & - & - & -\\
 \midrule
 \OUR  & 211.65 & 305.92 & 275.50 & 12.20 & 16.51 & 14.64 & 5.98 & 5.48 & 5.69\\

\bottomrule
\end{tabular}}
\end{table*}
