# Supplementary material for: Multimodal Motion Conditioned Diffusion Model for Skeleton-based Video Anomaly Detection
Source: arXiv:2307.07205 source file (2023-08-28)
Supplement: Supplementary file 6 [file models.tex]

\begin{table}[h]
\centering{

\caption{Ablation study on the number of timesteps of the diffusion process.}
\label{tab:models}
\resizebox{\linewidth}{!}{%
\begin{tabular}{lccc}
\toprule

  \textbf{Model } & \textbf{Params.} & \textbf{UBnormal} & \textbf{HR-UBnormal}\\ 
\midrule
 % w/o Motion Condition    &  54.11 &   54.98    \\
 % \hline
\OUR+MDM & 20M & 52.15 & 52.21   \\
 \OUR+MLD & 3.4M  & ON &  ON   \\ % 63.83 &  64.55
 \textbf{\OUR\ (proposed)} & 288K  & \textbf{\ubnres} &  \textbf{\hrubnres}      \\

\bottomrule
\end{tabular}}
}

\end{table}
